# Supplementary material for: Characterization of Maximally Random Jammed Sphere Packings: II. Correlation Functions and Density Fluctuations
Source: arXiv:1608.01984 ancillary file (2016-09-06)
Supplement: Supplementary file 1 [file supplementary-material-tables.pdf]

TABLE I: Probability and correlation functions of the equilibrium hard-sphere liquid with an average packing fraction  $\phi = 0.4780$  and a specific surface  $s = 2.868/D$ , where  $D$  is the diameter of a single sphere. The table lists for different distances  $r$  the functional values of the two-point correlation function  $S_2(r)$ , the surface-void correlation function  $F_{sv}(r)$  (where the void corresponds to the phase not covered by spheres), the surface-surface correlation function  $F_{ss}(r)$ , and the exclusion probability  $E_V(r)$ . If no statistical error are given in parentheses, they are smaller than the accuracy of the here presented data. For the correlation functions, they are below  $3 \cdot 10^{-4}$ . For the exclusion probability, they range mainly between  $2 \cdot 10^{-5}$  and  $10^{-7}$ .

| $r/D$ | $S_2(r)$ | $F_{sv}(r)/s$ | $F_{ss}(r)/s^2$ | $E_V(r)$ |
|-------|----------|---------------|-----------------|----------|
| 0     | 0.4780   | 1/2           | $\infty$        | 1        |
| 0.01  | 0.4709   | 0.5047        | 17.46           | 1.0000   |
| 0.02  | 0.4637   | 0.5090        | 8.768           | 1.0000   |
| 0.03  | 0.4566   | 0.5128        | 5.886           | 0.9999   |
| 0.04  | 0.4495   | 0.5162        | 4.456           | 0.9998   |
| 0.05  | 0.4424   | 0.5193        | 3.606           | 0.9995   |
| 0.06  | 0.4354   | 0.5219        | 3.046           | 0.9992   |
| 0.07  | 0.4285   | 0.5242        | 2.651           | 0.9987   |
| 0.08  | 0.4216   | 0.5262        | 2.359           | 0.9980   |
| 0.09  | 0.4148   | 0.5279        | 2.135           | 0.9972   |
| 0.10  | 0.4080   | 0.5294        | 1.959           | 0.9962   |
| 0.11  | 0.4014   | 0.5306        | 1.817           | 0.9949   |
| 0.12  | 0.3948   | 0.5315        | 1.702           | 0.9934   |
| 0.13  | 0.3884   | 0.5323        | 1.605           | 0.9916   |
| 0.14  | 0.3820   | 0.5328        | 1.525           | 0.9895   |
| 0.15  | 0.3758   | 0.5331        | 1.456           | 0.9871   |
| 0.16  | 0.3696   | 0.5333        | 1.398           | 0.9843   |
| 0.17  | 0.3636   | 0.5334        | 1.347           | 0.9812   |
| 0.18  | 0.3577   | 0.5332        | 1.303           | 0.9777   |
| 0.19  | 0.3518   | 0.5330        | 1.265           | 0.9738   |
| 0.20  | 0.3461   | 0.5326        | 1.231           | 0.9694   |
| 0.21  | 0.3406   | 0.5321        | 1.202           | 0.9646   |
| 0.22  | 0.3351   | 0.5315        | 1.175           | 0.9593   |
| 0.23  | 0.3298   | 0.5308        | 1.152           | 0.9535   |
| 0.24  | 0.3245   | 0.5301        | 1.131           | 0.9471   |
| 0.25  | 0.3194   | 0.5292        | 1.113           | 0.9403   |
| 0.26  | 0.3145   | 0.5283        | 1.096           | 0.9328   |
| 0.27  | 0.3096   | 0.5274        | 1.081           | 0.9247   |
| 0.28  | 0.3049   | 0.5263        | 1.068           | 0.9160   |
| 0.29  | 0.3003   | 0.5253        | 1.056           | 0.9067   |
| 0.30  | 0.2958   | 0.5242        | 1.045           | 0.8968   |
| 0.31  | 0.2915   | 0.5231        | 1.035           | 0.8861   |
| 0.32  | 0.2873   | 0.5219        | 1.026           | 0.8747   |
| 0.33  | 0.2832   | 0.5207        | 1.018           | 0.8626   |
| 0.34  | 0.2792   | 0.5196        | 1.011           | 0.8497   |
| 0.35  | 0.2754   | 0.5184        | 1.005           | 0.8360   |
| 0.36  | 0.2716   | 0.5172        | 0.999           | 0.8216   |
| 0.37  | 0.2680   | 0.5160        | 0.994           | 0.8063   |
| 0.38  | 0.2646   | 0.5148        | 0.989           | 0.7902   |
| 0.39  | 0.2612   | 0.5136        | 0.985           | 0.7731   |
| 0.40  | 0.2580   | 0.5125        | 0.981           | 0.7553   |
| 0.41  | 0.2548   | 0.5113        | 0.978           | 0.7364   |
| 0.42  | 0.2518   | 0.5102        | 0.975           | 0.7167   |
| 0.43  | 0.2489   | 0.5091        | 0.972           | 0.6960   |
| 0.44  | 0.2462   | 0.5081        | 0.970           | 0.6742   |
| 0.45  | 0.2435   | 0.5071        | 0.968           | 0.6515   |
| 0.46  | 0.2410   | 0.5061        | 0.966           | 0.6278   |
| 0.47  | 0.2385   | 0.5051        | 0.965           | 0.6030   |
| 0.48  | 0.2362   | 0.5042        | 0.963           | 0.5771   |
| 0.49  | 0.2340   | 0.5033        | 0.962           | 0.5501   |

|      |        |        |       |                         |
|------|--------|--------|-------|-------------------------|
| 0.50 | 0.2319 | 0.5025 | 0.962 | 0.5220                  |
| 0.51 | 0.2299 | 0.5018 | 0.961 | 0.4928                  |
| 0.52 | 0.2280 | 0.5010 | 0.961 | 0.4627                  |
| 0.53 | 0.2262 | 0.5004 | 0.961 | 0.4322                  |
| 0.54 | 0.2245 | 0.4998 | 0.961 | 0.4014                  |
| 0.55 | 0.2229 | 0.4992 | 0.961 | 0.3706                  |
| 0.56 | 0.2213 | 0.4988 | 0.961 | 0.3401                  |
| 0.57 | 0.2199 | 0.4983 | 0.962 | 0.3101                  |
| 0.58 | 0.2186 | 0.4980 | 0.962 | 0.2809                  |
| 0.59 | 0.2174 | 0.4977 | 0.963 | $2.53 \cdot 10^{-1}$    |
| 0.60 | 0.2163 | 0.4975 | 0.964 | $2.26 \cdot 10^{-1}$    |
| 0.61 | 0.2152 | 0.4973 | 0.965 | $2.00 \cdot 10^{-1}$    |
| 0.62 | 0.2143 | 0.4973 | 0.966 | $1.76 \cdot 10^{-1}$    |
| 0.63 | 0.2134 | 0.4972 | 0.968 | $1.54 \cdot 10^{-1}$    |
| 0.64 | 0.2126 | 0.4973 | 0.969 | $1.33 \cdot 10^{-1}$    |
| 0.65 | 0.2119 | 0.4975 | 0.971 | $1.14 \cdot 10^{-1}$    |
| 0.66 | 0.2113 | 0.4977 | 0.972 | $9.72 \cdot 10^{-2}$    |
| 0.67 | 0.2107 | 0.4980 | 0.974 | $8.21 \cdot 10^{-2}$    |
| 0.68 | 0.2103 | 0.4983 | 0.976 | $6.87 \cdot 10^{-2}$    |
| 0.69 | 0.2099 | 0.4988 | 0.978 | $5.69 \cdot 10^{-2}$    |
| 0.70 | 0.2096 | 0.4993 | 0.981 | $4.67 \cdot 10^{-2}$    |
| 0.71 | 0.2093 | 0.4999 | 0.983 | $3.79 \cdot 10^{-2}$    |
| 0.72 | 0.2092 | 0.5006 | 0.985 | $3.05 \cdot 10^{-2}$    |
| 0.73 | 0.2091 | 0.5014 | 0.988 | $2.43 \cdot 10^{-2}$    |
| 0.74 | 0.2090 | 0.5022 | 0.991 | $1.91 \cdot 10^{-2}$    |
| 0.75 | 0.2091 | 0.5031 | 0.994 | $1.49 \cdot 10^{-2}$    |
| 0.76 | 0.2092 | 0.5041 | 0.997 | $1.15 \cdot 10^{-2}$    |
| 0.77 | 0.2094 | 0.5052 | 1.000 | $8.76 \cdot 10^{-3}$    |
| 0.78 | 0.2096 | 0.5064 | 1.003 | $6.60 \cdot 10^{-3}$    |
| 0.79 | 0.2099 | 0.5076 | 1.006 | $4.91 \cdot 10^{-3}$    |
| 0.80 | 0.2103 | 0.5090 | 1.010 | $3.62 \cdot 10^{-3}$    |
| 0.81 | 0.2107 | 0.5104 | 1.013 | $2.63 \cdot 10^{-3}$    |
| 0.82 | 0.2112 | 0.5119 | 1.017 | $1.88 \cdot 10^{-3}$    |
| 0.83 | 0.2117 | 0.5134 | 1.021 | $1.34(1) \cdot 10^{-3}$ |
| 0.84 | 0.2123 | 0.5151 | 1.025 | $9.33(1) \cdot 10^{-4}$ |
| 0.85 | 0.2129 | 0.5168 | 1.029 | $6.44(8) \cdot 10^{-4}$ |
| 0.86 | 0.2137 | 0.5186 | 1.034 | $4.38(7) \cdot 10^{-4}$ |
| 0.87 | 0.2144 | 0.5205 | 1.038 | $2.94(5) \cdot 10^{-4}$ |
| 0.88 | 0.2152 | 0.5225 | 1.043 | $1.94(4) \cdot 10^{-4}$ |
| 0.89 | 0.2161 | 0.5245 | 1.048 | $1.26(4) \cdot 10^{-4}$ |
| 0.90 | 0.2170 | 0.5266 | 1.053 |                         |
| 0.91 | 0.2180 | 0.5288 | 1.058 |                         |
| 0.92 | 0.2190 | 0.5311 | 1.063 |                         |
| 0.93 | 0.2201 | 0.5335 | 1.068 |                         |
| 0.94 | 0.2212 | 0.5359 | 1.073 |                         |
| 0.95 | 0.2224 | 0.5384 | 1.079 |                         |
| 0.96 | 0.2236 | 0.5410 | 1.085 |                         |
| 0.97 | 0.2249 | 0.5436 | 1.091 |                         |
| 0.98 | 0.2262 | 0.5464 | 1.097 |                         |
| 0.99 | 0.2275 | 0.5492 | 1.103 |                         |
| 1.00 | 0.2289 | 0.5521 | 1.092 |                         |
| 1.01 | 0.2303 | 0.5501 | 0.942 |                         |
| 1.02 | 0.2316 | 0.5481 | 0.949 |                         |
| 1.03 | 0.2328 | 0.5463 | 0.955 |                         |
| 1.04 | 0.2339 | 0.5445 | 0.960 |                         |
| 1.05 | 0.2348 | 0.5428 | 0.965 |                         |
| 1.06 | 0.2357 | 0.5411 | 0.969 |                         |
| 1.07 | 0.2365 | 0.5395 | 0.972 |                         |
| 1.08 | 0.2372 | 0.5380 | 0.976 |                         |
| 1.09 | 0.2378 | 0.5366 | 0.978 |                         |
| 1.10 | 0.2383 | 0.5352 | 0.981 |                         |

|      |        |        |       |
|------|--------|--------|-------|
| 1.11 | 0.2388 | 0.5339 | 0.983 |
| 1.12 | 0.2391 | 0.5327 | 0.985 |
| 1.13 | 0.2394 | 0.5315 | 0.986 |
| 1.14 | 0.2396 | 0.5304 | 0.988 |
| 1.15 | 0.2397 | 0.5293 | 0.989 |
| 1.16 | 0.2397 | 0.5283 | 0.990 |
| 1.17 | 0.2397 | 0.5273 | 0.991 |
| 1.18 | 0.2396 | 0.5264 | 0.992 |
| 1.19 | 0.2395 | 0.5256 | 0.992 |
| 1.20 | 0.2393 | 0.5247 | 0.993 |
| 1.21 | 0.2391 | 0.5240 | 0.993 |
| 1.22 | 0.2388 | 0.5232 | 0.994 |
| 1.23 | 0.2385 | 0.5225 | 0.994 |
| 1.24 | 0.2382 | 0.5219 | 0.994 |
| 1.25 | 0.2378 | 0.5213 | 0.994 |
| 1.26 | 0.2374 | 0.5207 | 0.994 |
| 1.27 | 0.2369 | 0.5201 | 0.995 |
| 1.28 | 0.2364 | 0.5196 | 0.995 |
| 1.29 | 0.2360 | 0.5192 | 0.995 |
| 1.30 | 0.2355 | 0.5187 | 0.995 |
| 1.31 | 0.2349 | 0.5183 | 0.995 |
| 1.32 | 0.2344 | 0.5179 | 0.995 |
| 1.33 | 0.2339 | 0.5176 | 0.995 |
| 1.34 | 0.2333 | 0.5173 | 0.995 |
| 1.35 | 0.2328 | 0.5170 | 0.995 |
| 1.36 | 0.2323 | 0.5167 | 0.995 |
| 1.37 | 0.2317 | 0.5165 | 0.995 |
| 1.38 | 0.2312 | 0.5163 | 0.995 |
| 1.39 | 0.2307 | 0.5161 | 0.995 |
| 1.40 | 0.2301 | 0.5160 | 0.995 |
| 1.41 | 0.2296 | 0.5158 | 0.995 |
| 1.42 | 0.2291 | 0.5157 | 0.995 |
| 1.43 | 0.2287 | 0.5156 | 0.995 |
| 1.44 | 0.2282 | 0.5156 | 0.995 |
| 1.45 | 0.2277 | 0.5155 | 0.995 |
| 1.46 | 0.2273 | 0.5155 | 0.995 |
| 1.47 | 0.2269 | 0.5155 | 0.995 |
| 1.48 | 0.2265 | 0.5155 | 0.996 |
| 1.49 | 0.2261 | 0.5156 | 0.996 |
| 1.50 | 0.2258 | 0.5156 | 0.996 |
| 1.51 | 0.2255 | 0.5157 | 0.996 |
| 1.52 | 0.2251 | 0.5158 | 0.996 |
| 1.53 | 0.2249 | 0.5159 | 0.997 |
| 1.54 | 0.2246 | 0.5161 | 0.997 |
| 1.55 | 0.2244 | 0.5162 | 0.997 |
| 1.56 | 0.2242 | 0.5164 | 0.997 |
| 1.57 | 0.2240 | 0.5166 | 0.998 |
| 1.58 | 0.2238 | 0.5168 | 0.998 |
| 1.59 | 0.2237 | 0.5170 | 0.998 |
| 1.60 | 0.2236 | 0.5172 | 0.999 |
| 1.61 | 0.2235 | 0.5175 | 0.999 |
| 1.62 | 0.2234 | 0.5177 | 0.999 |
| 1.63 | 0.2234 | 0.5180 | 1.000 |
| 1.64 | 0.2234 | 0.5183 | 1.000 |
| 1.65 | 0.2234 | 0.5185 | 1.001 |
| 1.66 | 0.2234 | 0.5188 | 1.001 |
| 1.67 | 0.2235 | 0.5192 | 1.002 |
| 1.68 | 0.2235 | 0.5195 | 1.002 |
| 1.69 | 0.2236 | 0.5198 | 1.002 |
| 1.70 | 0.2237 | 0.5201 | 1.003 |
| 1.71 | 0.2239 | 0.5204 | 1.003 |
| 1.72 | 0.2240 | 0.5208 | 1.004 |

|      |        |        |       |
|------|--------|--------|-------|
| 1.73 | 0.2242 | 0.5211 | 1.004 |
| 1.74 | 0.2243 | 0.5214 | 1.005 |
| 1.75 | 0.2245 | 0.5218 | 1.005 |
| 1.76 | 0.2247 | 0.5221 | 1.005 |
| 1.77 | 0.2250 | 0.5225 | 1.006 |
| 1.78 | 0.2252 | 0.5228 | 1.006 |
| 1.79 | 0.2254 | 0.5231 | 1.006 |
| 1.80 | 0.2257 | 0.5234 | 1.007 |
| 1.81 | 0.2259 | 0.5238 | 1.007 |
| 1.82 | 0.2262 | 0.5241 | 1.007 |
| 1.83 | 0.2264 | 0.5244 | 1.007 |
| 1.84 | 0.2267 | 0.5247 | 1.007 |
| 1.85 | 0.2270 | 0.5249 | 1.007 |
| 1.86 | 0.2272 | 0.5252 | 1.007 |
| 1.87 | 0.2275 | 0.5254 | 1.007 |
| 1.88 | 0.2278 | 0.5257 | 1.007 |
| 1.89 | 0.2281 | 0.5259 | 1.007 |
| 1.90 | 0.2283 | 0.5261 | 1.007 |
| 1.91 | 0.2286 | 0.5262 | 1.007 |
| 1.92 | 0.2289 | 0.5264 | 1.006 |
| 1.93 | 0.2291 | 0.5265 | 1.006 |
| 1.94 | 0.2294 | 0.5266 | 1.005 |
| 1.95 | 0.2296 | 0.5267 | 1.005 |
| 1.96 | 0.2299 | 0.5267 | 1.004 |
| 1.97 | 0.2301 | 0.5267 | 1.003 |
| 1.98 | 0.2303 | 0.5267 | 1.003 |
| 1.99 | 0.2305 | 0.5266 | 1.002 |
| 2.00 | 0.2307 | 0.5265 | 1.001 |
| 2.01 | 0.2309 | 0.5264 | 1.000 |
| 2.02 | 0.2310 | 0.5262 | 0.999 |
| 2.03 | 0.2312 | 0.5260 | 0.998 |
| 2.04 | 0.2313 | 0.5258 | 0.998 |
| 2.05 | 0.2314 | 0.5256 | 0.997 |
| 2.06 | 0.2315 | 0.5253 | 0.997 |
| 2.07 | 0.2316 | 0.5251 | 0.997 |
| 2.08 | 0.2316 | 0.5248 | 0.997 |
| 2.09 | 0.2317 | 0.5245 | 0.996 |
| 2.10 | 0.2317 | 0.5242 | 0.996 |
| 2.11 | 0.2317 | 0.5239 | 0.996 |
| 2.12 | 0.2317 | 0.5236 | 0.996 |
| 2.13 | 0.2317 | 0.5234 | 0.996 |
| 2.14 | 0.2316 | 0.5231 | 0.996 |
| 2.15 | 0.2315 | 0.5228 | 0.996 |
| 2.16 | 0.2315 | 0.5225 | 0.996 |
| 2.17 | 0.2314 | 0.5223 | 0.996 |
| 2.18 | 0.2313 | 0.5220 | 0.996 |
| 2.19 | 0.2312 | 0.5218 | 0.996 |
| 2.20 | 0.2311 | 0.5216 | 0.997 |
| 2.21 | 0.2309 | 0.5213 | 0.997 |
| 2.22 | 0.2308 | 0.5211 | 0.997 |
| 2.23 | 0.2306 | 0.5209 | 0.997 |
| 2.24 | 0.2305 | 0.5208 | 0.997 |
| 2.25 | 0.2303 | 0.5206 | 0.997 |
| 2.26 | 0.2302 | 0.5204 | 0.997 |
| 2.27 | 0.2300 | 0.5203 | 0.997 |
| 2.28 | 0.2298 | 0.5201 | 0.997 |
| 2.29 | 0.2296 | 0.5200 | 0.997 |
| 2.30 | 0.2295 | 0.5199 | 0.998 |
| 2.31 | 0.2293 | 0.5198 | 0.998 |
| 2.32 | 0.2291 | 0.5197 | 0.998 |
| 2.33 | 0.2289 | 0.5197 | 0.998 |
| 2.34 | 0.2288 | 0.5196 | 0.998 |

|      |        |        |       |
|------|--------|--------|-------|
| 2.35 | 0.2286 | 0.5195 | 0.998 |
| 2.36 | 0.2284 | 0.5195 | 0.998 |
| 2.37 | 0.2283 | 0.5195 | 0.998 |
| 2.38 | 0.2281 | 0.5195 | 0.998 |
| 2.39 | 0.2280 | 0.5195 | 0.999 |
| 2.40 | 0.2278 | 0.5195 | 0.999 |
| 2.41 | 0.2277 | 0.5195 | 0.999 |
| 2.42 | 0.2276 | 0.5195 | 0.999 |
| 2.43 | 0.2274 | 0.5196 | 0.999 |
| 2.44 | 0.2273 | 0.5196 | 0.999 |
| 2.45 | 0.2272 | 0.5197 | 0.999 |
| 2.46 | 0.2271 | 0.5197 | 1.000 |
| 2.47 | 0.2270 | 0.5198 | 1.000 |
| 2.48 | 0.2270 | 0.5199 | 1.000 |
| 2.49 | 0.2269 | 0.5200 | 1.000 |
| 2.50 | 0.2268 | 0.5201 | 1.000 |
| 2.51 | 0.2268 | 0.5202 | 1.000 |
| 2.52 | 0.2267 | 0.5203 | 1.000 |
| 2.53 | 0.2267 | 0.5204 | 1.000 |
| 2.54 | 0.2267 | 0.5205 | 1.001 |
| 2.55 | 0.2267 | 0.5206 | 1.001 |
| 2.56 | 0.2267 | 0.5208 | 1.001 |
| 2.57 | 0.2267 | 0.5209 | 1.001 |
| 2.58 | 0.2267 | 0.5210 | 1.001 |
| 2.59 | 0.2267 | 0.5211 | 1.001 |
| 2.60 | 0.2267 | 0.5213 | 1.001 |
| 2.61 | 0.2268 | 0.5214 | 1.001 |
| 2.62 | 0.2268 | 0.5215 | 1.002 |
| 2.63 | 0.2268 | 0.5217 | 1.002 |
| 2.64 | 0.2269 | 0.5218 | 1.002 |
| 2.65 | 0.2270 | 0.5219 | 1.002 |
| 2.66 | 0.2270 | 0.5221 | 1.002 |
| 2.67 | 0.2271 | 0.5222 | 1.002 |
| 2.68 | 0.2272 | 0.5223 | 1.002 |
| 2.69 | 0.2273 | 0.5224 | 1.002 |
| 2.70 | 0.2274 | 0.5225 | 1.002 |
| 2.71 | 0.2275 | 0.5226 | 1.002 |
| 2.72 | 0.2275 | 0.5227 | 1.002 |
| 2.73 | 0.2276 | 0.5228 | 1.002 |
| 2.74 | 0.2277 | 0.5229 | 1.002 |
| 2.75 | 0.2278 | 0.5230 | 1.002 |
| 2.76 | 0.2279 | 0.5231 | 1.002 |
| 2.77 | 0.2280 | 0.5232 | 1.002 |
| 2.78 | 0.2282 | 0.5233 | 1.002 |
| 2.79 | 0.2283 | 0.5233 | 1.002 |
| 2.80 | 0.2284 | 0.5234 | 1.002 |
| 2.81 | 0.2285 | 0.5234 | 1.002 |
| 2.82 | 0.2286 | 0.5234 | 1.002 |
| 2.83 | 0.2286 | 0.5235 | 1.002 |
| 2.84 | 0.2287 | 0.5235 | 1.001 |
| 2.85 | 0.2288 | 0.5235 | 1.001 |
| 2.86 | 0.2289 | 0.5235 | 1.001 |
| 2.87 | 0.2290 | 0.5235 | 1.001 |
| 2.88 | 0.2291 | 0.5235 | 1.001 |
| 2.89 | 0.2292 | 0.5235 | 1.001 |
| 2.90 | 0.2292 | 0.5235 | 1.001 |
| 2.91 | 0.2293 | 0.5235 | 1.001 |
| 2.92 | 0.2294 | 0.5234 | 1.000 |
| 2.93 | 0.2294 | 0.5234 | 1.000 |
| 2.94 | 0.2295 | 0.5233 | 1.000 |
| 2.95 | 0.2295 | 0.5233 | 1.000 |
| 2.96 | 0.2296 | 0.5232 | 1.000 |

|      |        |        |       |
|------|--------|--------|-------|
| 2.97 | 0.2296 | 0.5232 | 1.000 |
| 2.98 | 0.2296 | 0.5231 | 1.000 |
| 2.99 | 0.2296 | 0.5230 | 0.999 |
| 3.00 | 0.2297 | 0.5229 | 0.999 |
| 3.01 | 0.2297 | 0.5229 | 0.999 |
| 3.02 | 0.2297 | 0.5228 | 0.999 |
| 3.03 | 0.2297 | 0.5227 | 0.999 |
| 3.04 | 0.2297 | 0.5226 | 0.999 |
| 3.05 | 0.2297 | 0.5225 | 0.999 |
| 3.06 | 0.2296 | 0.5224 | 0.999 |
| 3.07 | 0.2296 | 0.5223 | 0.999 |
| 3.08 | 0.2296 | 0.5222 | 0.999 |
| 3.09 | 0.2296 | 0.5221 | 0.999 |
| 3.10 | 0.2295 | 0.5221 | 0.999 |
| 3.11 | 0.2295 | 0.5220 | 0.999 |
| 3.12 | 0.2294 | 0.5219 | 0.999 |
| 3.13 | 0.2294 | 0.5218 | 0.999 |
| 3.14 | 0.2293 | 0.5217 | 0.999 |
| 3.15 | 0.2293 | 0.5216 | 0.999 |
| 3.16 | 0.2292 | 0.5216 | 0.999 |
| 3.17 | 0.2292 | 0.5215 | 0.999 |
| 3.18 | 0.2291 | 0.5214 | 0.999 |
| 3.19 | 0.2291 | 0.5214 | 0.999 |
| 3.20 | 0.2290 | 0.5213 | 0.999 |
| 3.21 | 0.2289 | 0.5212 | 0.999 |
| 3.22 | 0.2289 | 0.5212 | 0.999 |
| 3.23 | 0.2288 | 0.5211 | 0.999 |
| 3.24 | 0.2287 | 0.5211 | 0.999 |
| 3.25 | 0.2287 | 0.5211 | 0.999 |
| 3.26 | 0.2286 | 0.5210 | 0.999 |
| 3.27 | 0.2285 | 0.5210 | 0.999 |
| 3.28 | 0.2285 | 0.5210 | 0.999 |
| 3.29 | 0.2284 | 0.5210 | 0.999 |
| 3.30 | 0.2284 | 0.5210 | 0.999 |
| 3.31 | 0.2283 | 0.5210 | 0.999 |
| 3.32 | 0.2282 | 0.5210 | 0.999 |
| 3.33 | 0.2282 | 0.5210 | 0.999 |
| 3.34 | 0.2281 | 0.5210 | 1.000 |
| 3.35 | 0.2281 | 0.5210 | 1.000 |
| 3.36 | 0.2280 | 0.5210 | 1.000 |
| 3.37 | 0.2280 | 0.5210 | 1.000 |
| 3.38 | 0.2280 | 0.5211 | 1.000 |
| 3.39 | 0.2279 | 0.5211 | 1.000 |
| 3.40 | 0.2279 | 0.5211 | 1.000 |
| 3.41 | 0.2279 | 0.5212 | 1.000 |
| 3.42 | 0.2278 | 0.5212 | 1.000 |
| 3.43 | 0.2278 | 0.5212 | 1.000 |
| 3.44 | 0.2278 | 0.5213 | 1.000 |
| 3.45 | 0.2278 | 0.5213 | 1.000 |
| 3.46 | 0.2278 | 0.5214 | 1.000 |
| 3.47 | 0.2278 | 0.5214 | 1.000 |
| 3.48 | 0.2278 | 0.5215 | 1.000 |
| 3.49 | 0.2278 | 0.5215 | 1.001 |
| 3.50 | 0.2278 | 0.5216 | 1.001 |
| 3.51 | 0.2278 | 0.5217 | 1.001 |
| 3.52 | 0.2278 | 0.5217 | 1.001 |
| 3.53 | 0.2278 | 0.5218 | 1.001 |
| 3.54 | 0.2278 | 0.5218 | 1.001 |
| 3.55 | 0.2278 | 0.5219 | 1.001 |
| 3.56 | 0.2279 | 0.5219 | 1.001 |
| 3.57 | 0.2279 | 0.5220 | 1.001 |
| 3.58 | 0.2279 | 0.5220 | 1.001 |

|      |        |        |       |
|------|--------|--------|-------|
| 3.59 | 0.2280 | 0.5221 | 1.001 |
| 3.60 | 0.2280 | 0.5221 | 1.001 |
| 3.61 | 0.2280 | 0.5222 | 1.001 |
| 3.62 | 0.2281 | 0.5222 | 1.001 |
| 3.63 | 0.2281 | 0.5223 | 1.001 |
| 3.64 | 0.2281 | 0.5223 | 1.001 |
| 3.65 | 0.2282 | 0.5224 | 1.001 |
| 3.66 | 0.2282 | 0.5224 | 1.001 |
| 3.67 | 0.2283 | 0.5224 | 1.001 |
| 3.68 | 0.2283 | 0.5225 | 1.001 |
| 3.69 | 0.2283 | 0.5225 | 1.001 |
| 3.70 | 0.2284 | 0.5225 | 1.001 |
| 3.71 | 0.2284 | 0.5225 | 1.001 |
| 3.72 | 0.2285 | 0.5226 | 1.001 |
| 3.73 | 0.2285 | 0.5226 | 1.001 |
| 3.74 | 0.2285 | 0.5226 | 1.001 |
| 3.75 | 0.2286 | 0.5226 | 1.001 |
| 3.76 | 0.2286 | 0.5226 | 1.000 |
| 3.77 | 0.2287 | 0.5226 | 1.000 |
| 3.78 | 0.2287 | 0.5226 | 1.000 |
| 3.79 | 0.2287 | 0.5226 | 1.000 |
| 3.80 | 0.2288 | 0.5226 | 1.000 |
| 3.81 | 0.2288 | 0.5226 | 1.000 |
| 3.82 | 0.2288 | 0.5226 | 1.000 |
| 3.83 | 0.2288 | 0.5226 | 1.000 |
| 3.84 | 0.2289 | 0.5226 | 1.000 |
| 3.85 | 0.2289 | 0.5225 | 1.000 |
| 3.86 | 0.2289 | 0.5225 | 1.000 |
| 3.87 | 0.2289 | 0.5225 | 1.000 |
| 3.88 | 0.2289 | 0.5225 | 1.000 |
| 3.89 | 0.2290 | 0.5224 | 1.000 |
| 3.90 | 0.2290 | 0.5224 | 1.000 |
| 3.91 | 0.2290 | 0.5224 | 1.000 |
| 3.92 | 0.2290 | 0.5223 | 1.000 |
| 3.93 | 0.2290 | 0.5223 | 1.000 |
| 3.94 | 0.2290 | 0.5223 | 1.000 |
| 3.95 | 0.2290 | 0.5222 | 1.000 |
| 3.96 | 0.2290 | 0.5222 | 1.000 |
| 3.97 | 0.2290 | 0.5222 | 1.000 |
| 3.98 | 0.2290 | 0.5221 | 1.000 |
| 3.99 | 0.2290 | 0.5221 | 1.000 |
| 4.00 | 0.2290 | 0.5221 | 1.000 |
| 4.01 | 0.2289 | 0.5220 | 0.999 |
| 4.02 | 0.2289 | 0.5220 | 0.999 |
| 4.03 | 0.2289 | 0.5220 | 0.999 |
| 4.04 | 0.2289 | 0.5219 | 0.999 |
| 4.05 | 0.2289 | 0.5219 | 0.999 |
| 4.06 | 0.2288 | 0.5219 | 0.999 |
| 4.07 | 0.2288 | 0.5218 | 0.999 |
| 4.08 | 0.2288 | 0.5218 | 0.999 |
| 4.09 | 0.2288 | 0.5218 | 0.999 |
| 4.10 | 0.2288 | 0.5217 | 0.999 |
| 4.11 | 0.2287 | 0.5217 | 0.999 |
| 4.12 | 0.2287 | 0.5217 | 0.999 |
| 4.13 | 0.2287 | 0.5217 | 0.999 |
| 4.14 | 0.2286 | 0.5216 | 0.999 |
| 4.15 | 0.2286 | 0.5216 | 1.000 |
| 4.16 | 0.2286 | 0.5216 | 1.000 |
| 4.17 | 0.2286 | 0.5216 | 1.000 |
| 4.18 | 0.2285 | 0.5216 | 1.000 |
| 4.19 | 0.2285 | 0.5216 | 1.000 |
| 4.20 | 0.2285 | 0.5216 | 1.000 |

|          |        |        |       |
|----------|--------|--------|-------|
| 4.21     | 0.2285 | 0.5216 | 1.000 |
| 4.22     | 0.2284 | 0.5215 | 1.000 |
| 4.23     | 0.2284 | 0.5215 | 1.000 |
| $\infty$ | 0.2285 | 0.5220 | 1     |

TABLE II: Probability and correlation functions of the MRJ hard-sphere packings with an average packing fraction  $\phi = 0.6356$  and a specific surface  $s = 3.814/D$ , where  $D$  is the diameter of a single sphere. The table lists for different distances  $r$  the functional values of the two-point correlation function  $S_2(r)$ , the surface-void correlation function  $F_{sv}(r)$  (where the void corresponds to the phase not covered by spheres), the surface-surface correlation function  $F_{ss}(r)$ , and the exclusion probability  $E_V(r)$ . If no statistical error are given in parentheses, they are smaller than the accuracy of the here presented data. For the correlation functions, they are below  $2 \cdot 10^{-4}$ . For the exclusion probability, they range mainly between  $5 \cdot 10^{-6}$  and  $10^{-7}$ .

| $r/D$ | $S_2(r)$ | $F_{sv}(r)/s$ | $F_{ss}(r)/s^2$ | $E_V(r)$ |
|-------|----------|---------------|-----------------|----------|
| 0     | 0.6356   | 1/2           | $\infty$        | 1        |
| 0.01  | 0.6261   | 0.4972        | 13.53           | 1.0000   |
| 0.02  | 0.6169   | 0.4940        | 6.991           | 1.0000   |
| 0.03  | 0.6079   | 0.4906        | 4.819           | 0.9999   |
| 0.04  | 0.5991   | 0.4870        | 3.737           | 0.9997   |
| 0.05  | 0.5905   | 0.4834        | 3.092           | 0.9994   |
| 0.06  | 0.5821   | 0.4796        | 2.663           | 0.9989   |
| 0.07  | 0.5740   | 0.4758        | 2.359           | 0.9983   |
| 0.08  | 0.5660   | 0.4719        | 2.133           | 0.9974   |
| 0.09  | 0.5583   | 0.4680        | 1.958           | 0.9963   |
| 0.10  | 0.5508   | 0.4641        | 1.819           | 0.9949   |
| 0.11  | 0.5435   | 0.4601        | 1.706           | 0.9932   |
| 0.12  | 0.5364   | 0.4562        | 1.613           | 0.9912   |
| 0.13  | 0.5296   | 0.4522        | 1.535           | 0.9888   |
| 0.14  | 0.5229   | 0.4483        | 1.469           | 0.9860   |
| 0.15  | 0.5164   | 0.4444        | 1.412           | 0.9828   |
| 0.16  | 0.5102   | 0.4405        | 1.363           | 0.9792   |
| 0.17  | 0.5042   | 0.4366        | 1.320           | 0.9750   |
| 0.18  | 0.4983   | 0.4328        | 1.282           | 0.9703   |
| 0.19  | 0.4927   | 0.4290        | 1.248           | 0.9651   |
| 0.20  | 0.4872   | 0.4252        | 1.219           | 0.9593   |
| 0.21  | 0.4819   | 0.4215        | 1.192           | 0.9529   |
| 0.22  | 0.4769   | 0.4179        | 1.168           | 0.9459   |
| 0.23  | 0.4720   | 0.4143        | 1.147           | 0.9381   |
| 0.24  | 0.4673   | 0.4107        | 1.127           | 0.9297   |
| 0.25  | 0.4628   | 0.4073        | 1.110           | 0.9206   |
| 0.26  | 0.4584   | 0.4039        | 1.094           | 0.9106   |
| 0.27  | 0.4542   | 0.4005        | 1.080           | 0.8999   |
| 0.28  | 0.4502   | 0.3973        | 1.066           | 0.8884   |
| 0.29  | 0.4464   | 0.3941        | 1.054           | 0.8760   |
| 0.30  | 0.4427   | 0.3909        | 1.043           | 0.8627   |
| 0.31  | 0.4392   | 0.3879        | 1.033           | 0.8485   |
| 0.32  | 0.4358   | 0.3849        | 1.024           | 0.8334   |
| 0.33  | 0.4326   | 0.3820        | 1.015           | 0.8173   |



|      |        |        |       |                         |
|------|--------|--------|-------|-------------------------|
| 0.34 | 0.4295 | 0.3792 | 1.008 | 0.8002                  |
| 0.35 | 0.4266 | 0.3765 | 1.001 | 0.7820                  |
| 0.36 | 0.4238 | 0.3739 | 0.994 | 0.7628                  |
| 0.37 | 0.4212 | 0.3713 | 0.988 | 0.7425                  |
| 0.38 | 0.4187 | 0.3689 | 0.982 | 0.7210                  |
| 0.39 | 0.4163 | 0.3665 | 0.977 | 0.6984                  |
| 0.40 | 0.4141 | 0.3643 | 0.973 | 0.6746                  |
| 0.41 | 0.4119 | 0.3621 | 0.969 | 0.6496                  |
| 0.42 | 0.4099 | 0.3600 | 0.965 | 0.6233                  |
| 0.43 | 0.4080 | 0.3580 | 0.961 | 0.5957                  |
| 0.44 | 0.4063 | 0.3561 | 0.958 | 0.5669                  |
| 0.45 | 0.4046 | 0.3543 | 0.955 | 0.5367                  |
| 0.46 | 0.4031 | 0.3526 | 0.953 | 0.5051                  |
| 0.47 | 0.4016 | 0.3510 | 0.951 | 0.4721                  |
| 0.48 | 0.4003 | 0.3496 | 0.949 | 0.4377                  |
| 0.49 | 0.3990 | 0.3482 | 0.947 | 0.4018                  |
| 0.50 | 0.3979 | 0.3469 | 0.945 | 0.3644                  |
| 0.51 | 0.3968 | 0.3457 | 0.944 | 0.3268                  |
| 0.52 | 0.3958 | 0.3446 | 0.943 | 0.2904                  |
| 0.53 | 0.3950 | 0.3436 | 0.942 | 0.2555                  |
| 0.54 | 0.3942 | 0.3427 | 0.942 | 0.2225                  |
| 0.55 | 0.3934 | 0.3419 | 0.941 | 0.1916                  |
| 0.56 | 0.3928 | 0.3412 | 0.941 | 0.1630                  |
| 0.57 | 0.3922 | 0.3407 | 0.941 | 0.1370                  |
| 0.58 | 0.3917 | 0.3402 | 0.942 | 0.1138                  |
| 0.59 | 0.3913 | 0.3398 | 0.942 | $9.35 \cdot 10^{-2}$    |
| 0.60 | 0.3909 | 0.3395 | 0.943 | $7.60 \cdot 10^{-2}$    |
| 0.61 | 0.3906 | 0.3394 | 0.943 | $6.09 \cdot 10^{-2}$    |
| 0.62 | 0.3904 | 0.3393 | 0.944 | $4.83 \cdot 10^{-2}$    |
| 0.63 | 0.3902 | 0.3393 | 0.945 | $3.77 \cdot 10^{-2}$    |
| 0.64 | 0.3900 | 0.3394 | 0.947 | $2.90 \cdot 10^{-2}$    |
| 0.65 | 0.3900 | 0.3397 | 0.948 | $2.19 \cdot 10^{-2}$    |
| 0.66 | 0.3899 | 0.3400 | 0.950 | $1.63 \cdot 10^{-2}$    |
| 0.67 | 0.3899 | 0.3404 | 0.952 | $1.20 \cdot 10^{-2}$    |
| 0.68 | 0.3900 | 0.3409 | 0.954 | $8.60 \cdot 10^{-3}$    |
| 0.69 | 0.3901 | 0.3415 | 0.957 | $6.10 \cdot 10^{-3}$    |
| 0.70 | 0.3903 | 0.3422 | 0.959 | $4.26 \cdot 10^{-3}$    |
| 0.71 | 0.3905 | 0.3429 | 0.962 | $2.93 \cdot 10^{-3}$    |
| 0.72 | 0.3907 | 0.3438 | 0.965 | $1.99 \cdot 10^{-3}$    |
| 0.73 | 0.3910 | 0.3447 | 0.968 | $1.32 \cdot 10^{-3}$    |
| 0.74 | 0.3913 | 0.3457 | 0.972 | $8.64 \cdot 10^{-4}$    |
| 0.75 | 0.3917 | 0.3468 | 0.976 | $5.53 \cdot 10^{-4}$    |
| 0.76 | 0.3921 | 0.3480 | 0.980 | $3.47 \cdot 10^{-4}$    |
| 0.77 | 0.3925 | 0.3492 | 0.984 | $2.13 \cdot 10^{-4}$    |
| 0.78 | 0.3929 | 0.3505 | 0.988 | $1.28 \cdot 10^{-4}$    |
| 0.79 | 0.3934 | 0.3518 | 0.993 | $7.53 \cdot 10^{-5}$    |
| 0.80 | 0.3939 | 0.3532 | 0.997 | $4.34 \cdot 10^{-5}$    |
| 0.81 | 0.3945 | 0.3547 | 1.002 | $2.45 \cdot 10^{-5}$    |
| 0.82 | 0.3951 | 0.3563 | 1.007 | $1.36 \cdot 10^{-5}$    |
| 0.83 | 0.3957 | 0.3579 | 1.013 | $7.49(3) \cdot 10^{-6}$ |
| 0.84 | 0.3964 | 0.3595 | 1.018 | $4.02(2) \cdot 10^{-6}$ |
| 0.85 | 0.3970 | 0.3613 | 1.024 | $2.09(1) \cdot 10^{-6}$ |
| 0.86 | 0.3977 | 0.3631 | 1.029 | $1.08(1) \cdot 10^{-6}$ |
| 0.87 | 0.3985 | 0.3650 | 1.035 | $5.47(7) \cdot 10^{-7}$ |
| 0.88 | 0.3993 | 0.3669 | 1.041 | $2.74(5) \cdot 10^{-7}$ |
| 0.89 | 0.4000 | 0.3689 | 1.047 | $1.33(4) \cdot 10^{-7}$ |
| 0.90 | 0.4009 | 0.3710 | 1.053 |                         |
| 0.91 | 0.4017 | 0.3732 | 1.060 |                         |
| 0.92 | 0.4026 | 0.3754 | 1.066 |                         |
| 0.93 | 0.4035 | 0.3777 | 1.073 |                         |
| 0.94 | 0.4044 | 0.3800 | 1.079 |                         |

|      |        |        |       |
|------|--------|--------|-------|
| 0.95 | 0.4053 | 0.3825 | 1.086 |
| 0.96 | 0.4063 | 0.3850 | 1.093 |
| 0.97 | 0.4073 | 0.3876 | 1.101 |
| 0.98 | 0.4083 | 0.3903 | 1.108 |
| 0.99 | 0.4094 | 0.3930 | 1.116 |
| 1.00 | 0.4104 | 0.3958 | 1.007 |
| 1.01 | 0.4114 | 0.3937 | 0.993 |
| 1.02 | 0.4122 | 0.3916 | 0.994 |
| 1.03 | 0.4129 | 0.3896 | 0.994 |
| 1.04 | 0.4134 | 0.3877 | 0.994 |
| 1.05 | 0.4139 | 0.3859 | 0.994 |
| 1.06 | 0.4141 | 0.3841 | 0.994 |
| 1.07 | 0.4143 | 0.3823 | 0.994 |
| 1.08 | 0.4144 | 0.3807 | 0.993 |
| 1.09 | 0.4144 | 0.3790 | 0.993 |
| 1.10 | 0.4143 | 0.3775 | 0.992 |
| 1.11 | 0.4141 | 0.3760 | 0.992 |
| 1.12 | 0.4138 | 0.3746 | 0.992 |
| 1.13 | 0.4135 | 0.3732 | 0.991 |
| 1.14 | 0.4132 | 0.3719 | 0.991 |
| 1.15 | 0.4127 | 0.3706 | 0.990 |
| 1.16 | 0.4123 | 0.3694 | 0.990 |
| 1.17 | 0.4118 | 0.3682 | 0.989 |
| 1.18 | 0.4113 | 0.3671 | 0.989 |
| 1.19 | 0.4107 | 0.3661 | 0.988 |
| 1.20 | 0.4102 | 0.3651 | 0.988 |
| 1.21 | 0.4096 | 0.3641 | 0.987 |
| 1.22 | 0.4090 | 0.3633 | 0.987 |
| 1.23 | 0.4084 | 0.3624 | 0.987 |
| 1.24 | 0.4078 | 0.3616 | 0.986 |
| 1.25 | 0.4072 | 0.3609 | 0.986 |
| 1.26 | 0.4067 | 0.3602 | 0.986 |
| 1.27 | 0.4061 | 0.3596 | 0.986 |
| 1.28 | 0.4055 | 0.3590 | 0.985 |
| 1.29 | 0.4050 | 0.3585 | 0.985 |
| 1.30 | 0.4044 | 0.3580 | 0.985 |
| 1.31 | 0.4039 | 0.3576 | 0.985 |
| 1.32 | 0.4034 | 0.3572 | 0.985 |
| 1.33 | 0.4029 | 0.3568 | 0.985 |
| 1.34 | 0.4025 | 0.3565 | 0.985 |
| 1.35 | 0.4021 | 0.3563 | 0.985 |
| 1.36 | 0.4017 | 0.3561 | 0.985 |
| 1.37 | 0.4013 | 0.3559 | 0.985 |
| 1.38 | 0.4009 | 0.3558 | 0.985 |
| 1.39 | 0.4006 | 0.3557 | 0.985 |
| 1.40 | 0.4003 | 0.3557 | 0.986 |
| 1.41 | 0.4001 | 0.3557 | 0.986 |
| 1.42 | 0.3998 | 0.3557 | 0.986 |
| 1.43 | 0.3996 | 0.3558 | 0.987 |
| 1.44 | 0.3995 | 0.3559 | 0.987 |
| 1.45 | 0.3993 | 0.3561 | 0.988 |
| 1.46 | 0.3992 | 0.3562 | 0.988 |
| 1.47 | 0.3991 | 0.3564 | 0.989 |
| 1.48 | 0.3991 | 0.3567 | 0.989 |
| 1.49 | 0.3990 | 0.3570 | 0.990 |
| 1.50 | 0.3990 | 0.3572 | 0.991 |
| 1.51 | 0.3991 | 0.3576 | 0.991 |
| 1.52 | 0.3991 | 0.3579 | 0.992 |
| 1.53 | 0.3992 | 0.3583 | 0.993 |
| 1.54 | 0.3992 | 0.3587 | 0.994 |
| 1.55 | 0.3994 | 0.3591 | 0.995 |
| 1.56 | 0.3995 | 0.3595 | 0.996 |

|      |        |        |       |
|------|--------|--------|-------|
| 1.57 | 0.3996 | 0.3599 | 0.997 |
| 1.58 | 0.3998 | 0.3604 | 0.998 |
| 1.59 | 0.4000 | 0.3608 | 0.999 |
| 1.60 | 0.4002 | 0.3613 | 1.000 |
| 1.61 | 0.4004 | 0.3618 | 1.001 |
| 1.62 | 0.4006 | 0.3623 | 1.002 |
| 1.63 | 0.4008 | 0.3628 | 1.003 |
| 1.64 | 0.4011 | 0.3633 | 1.004 |
| 1.65 | 0.4013 | 0.3637 | 1.005 |
| 1.66 | 0.4016 | 0.3642 | 1.007 |
| 1.67 | 0.4018 | 0.3647 | 1.008 |
| 1.68 | 0.4021 | 0.3652 | 1.009 |
| 1.69 | 0.4024 | 0.3657 | 1.010 |
| 1.70 | 0.4026 | 0.3661 | 1.011 |
| 1.71 | 0.4029 | 0.3666 | 1.012 |
| 1.72 | 0.4032 | 0.3670 | 1.012 |
| 1.73 | 0.4034 | 0.3675 | 1.013 |
| 1.74 | 0.4037 | 0.3679 | 1.014 |
| 1.75 | 0.4040 | 0.3683 | 1.014 |
| 1.76 | 0.4042 | 0.3686 | 1.014 |
| 1.77 | 0.4045 | 0.3690 | 1.014 |
| 1.78 | 0.4047 | 0.3693 | 1.015 |
| 1.79 | 0.4049 | 0.3696 | 1.015 |
| 1.80 | 0.4052 | 0.3699 | 1.015 |
| 1.81 | 0.4054 | 0.3702 | 1.014 |
| 1.82 | 0.4056 | 0.3704 | 1.014 |
| 1.83 | 0.4058 | 0.3706 | 1.014 |
| 1.84 | 0.4060 | 0.3708 | 1.013 |
| 1.85 | 0.4062 | 0.3709 | 1.013 |
| 1.86 | 0.4063 | 0.3710 | 1.012 |
| 1.87 | 0.4065 | 0.3711 | 1.012 |
| 1.88 | 0.4066 | 0.3711 | 1.011 |
| 1.89 | 0.4068 | 0.3711 | 1.010 |
| 1.90 | 0.4069 | 0.3711 | 1.009 |
| 1.91 | 0.4070 | 0.3710 | 1.008 |
| 1.92 | 0.4071 | 0.3708 | 1.007 |
| 1.93 | 0.4072 | 0.3706 | 1.006 |
| 1.94 | 0.4072 | 0.3704 | 1.004 |
| 1.95 | 0.4072 | 0.3701 | 1.003 |
| 1.96 | 0.4073 | 0.3698 | 1.001 |
| 1.97 | 0.4072 | 0.3694 | 0.999 |
| 1.98 | 0.4072 | 0.3689 | 0.997 |
| 1.99 | 0.4072 | 0.3684 | 0.995 |
| 2.00 | 0.4071 | 0.3678 | 0.993 |
| 2.01 | 0.4070 | 0.3672 | 0.993 |
| 2.02 | 0.4069 | 0.3666 | 0.992 |
| 2.03 | 0.4067 | 0.3661 | 0.992 |
| 2.04 | 0.4066 | 0.3655 | 0.992 |
| 2.05 | 0.4064 | 0.3650 | 0.992 |
| 2.06 | 0.4062 | 0.3645 | 0.992 |
| 2.07 | 0.4060 | 0.3640 | 0.992 |
| 2.08 | 0.4058 | 0.3636 | 0.992 |
| 2.09 | 0.4055 | 0.3632 | 0.992 |
| 2.10 | 0.4053 | 0.3628 | 0.992 |
| 2.11 | 0.4051 | 0.3625 | 0.992 |
| 2.12 | 0.4049 | 0.3621 | 0.992 |
| 2.13 | 0.4046 | 0.3618 | 0.992 |
| 2.14 | 0.4044 | 0.3616 | 0.992 |
| 2.15 | 0.4042 | 0.3613 | 0.992 |
| 2.16 | 0.4040 | 0.3611 | 0.992 |
| 2.17 | 0.4037 | 0.3609 | 0.992 |
| 2.18 | 0.4035 | 0.3607 | 0.992 |

|      |        |        |       |
|------|--------|--------|-------|
| 2.19 | 0.4033 | 0.3606 | 0.992 |
| 2.20 | 0.4032 | 0.3605 | 0.993 |
| 2.21 | 0.4030 | 0.3604 | 0.993 |
| 2.22 | 0.4028 | 0.3603 | 0.993 |
| 2.23 | 0.4026 | 0.3603 | 0.993 |
| 2.24 | 0.4025 | 0.3603 | 0.994 |
| 2.25 | 0.4024 | 0.3603 | 0.994 |
| 2.26 | 0.4022 | 0.3603 | 0.994 |
| 2.27 | 0.4021 | 0.3604 | 0.994 |
| 2.28 | 0.4020 | 0.3604 | 0.995 |
| 2.29 | 0.4020 | 0.3605 | 0.995 |
| 2.30 | 0.4019 | 0.3606 | 0.996 |
| 2.31 | 0.4018 | 0.3608 | 0.996 |
| 2.32 | 0.4018 | 0.3609 | 0.996 |
| 2.33 | 0.4018 | 0.3611 | 0.997 |
| 2.34 | 0.4018 | 0.3612 | 0.997 |
| 2.35 | 0.4018 | 0.3614 | 0.998 |
| 2.36 | 0.4018 | 0.3616 | 0.998 |
| 2.37 | 0.4018 | 0.3618 | 0.998 |
| 2.38 | 0.4018 | 0.3620 | 0.999 |
| 2.39 | 0.4019 | 0.3622 | 0.999 |
| 2.40 | 0.4019 | 0.3625 | 1.000 |
| 2.41 | 0.4020 | 0.3627 | 1.000 |
| 2.42 | 0.4021 | 0.3629 | 1.001 |
| 2.43 | 0.4022 | 0.3632 | 1.001 |
| 2.44 | 0.4022 | 0.3634 | 1.002 |
| 2.45 | 0.4023 | 0.3637 | 1.002 |
| 2.46 | 0.4025 | 0.3639 | 1.002 |
| 2.47 | 0.4026 | 0.3641 | 1.003 |
| 2.48 | 0.4027 | 0.3644 | 1.003 |
| 2.49 | 0.4028 | 0.3646 | 1.004 |
| 2.50 | 0.4029 | 0.3649 | 1.004 |
| 2.51 | 0.4031 | 0.3651 | 1.004 |
| 2.52 | 0.4032 | 0.3653 | 1.005 |
| 2.53 | 0.4033 | 0.3655 | 1.005 |
| 2.54 | 0.4034 | 0.3657 | 1.005 |
| 2.55 | 0.4036 | 0.3659 | 1.005 |
| 2.56 | 0.4037 | 0.3661 | 1.005 |
| 2.57 | 0.4038 | 0.3663 | 1.006 |
| 2.58 | 0.4040 | 0.3664 | 1.006 |
| 2.59 | 0.4041 | 0.3666 | 1.006 |
| 2.60 | 0.4042 | 0.3667 | 1.006 |
| 2.61 | 0.4043 | 0.3668 | 1.006 |
| 2.62 | 0.4044 | 0.3670 | 1.006 |
| 2.63 | 0.4045 | 0.3670 | 1.006 |
| 2.64 | 0.4046 | 0.3671 | 1.005 |
| 2.65 | 0.4047 | 0.3672 | 1.005 |
| 2.66 | 0.4048 | 0.3672 | 1.005 |
| 2.67 | 0.4049 | 0.3673 | 1.005 |
| 2.68 | 0.4050 | 0.3673 | 1.004 |
| 2.69 | 0.4051 | 0.3673 | 1.004 |
| 2.70 | 0.4051 | 0.3672 | 1.004 |
| 2.71 | 0.4052 | 0.3672 | 1.003 |
| 2.72 | 0.4052 | 0.3671 | 1.003 |
| 2.73 | 0.4053 | 0.3671 | 1.003 |
| 2.74 | 0.4053 | 0.3670 | 1.002 |
| 2.75 | 0.4053 | 0.3669 | 1.002 |
| 2.76 | 0.4053 | 0.3668 | 1.002 |
| 2.77 | 0.4054 | 0.3667 | 1.001 |
| 2.78 | 0.4054 | 0.3666 | 1.001 |
| 2.79 | 0.4053 | 0.3664 | 1.000 |
| 2.80 | 0.4053 | 0.3663 | 1.000 |

|          |        |        |       |
|----------|--------|--------|-------|
| 2.81     | 0.4053 | 0.3662 | 1.000 |
| 2.82     | 0.4053 | 0.3660 | 0.999 |
| 2.83     | 0.4052 | 0.3658 | 0.999 |
| $\infty$ | 0.4040 | 0.3644 | 1     |

TABLE III: Spectral density (i.e., the Fourier transform of the covariance  $\chi_V(r) = S_2(r) - \phi^2$ ) of the equilibrium hard-sphere liquid. It is derived from the direct Fourier transformation of the periodic simulation box. The allowed values of the wave vector are binned w.r.t. their absolute value  $k$  and the resulting spectral densities are then averaged over 100 different packings. The third column displays the standard error of the mean.

| $k \cdot D$ | $\tilde{\chi}_V(k)/D^3$ | $\sigma[\tilde{\chi}_V(k)]/D^3$ |
|-------------|-------------------------|---------------------------------|
| 0.3         | $5.68 \cdot 10^{-3}$    | $2 \cdot 10^{-4}$               |
| 0.6         | $5.40 \cdot 10^{-3}$    | $1 \cdot 10^{-4}$               |
| 0.8         | $5.65 \cdot 10^{-3}$    | $1 \cdot 10^{-4}$               |
| 1.1         | $5.60 \cdot 10^{-3}$    | $1 \cdot 10^{-4}$               |
| 1.4         | $5.75 \cdot 10^{-3}$    | $8 \cdot 10^{-5}$               |
| 1.7         | $5.88 \cdot 10^{-3}$    | $7 \cdot 10^{-5}$               |
| 2.0         | $5.87 \cdot 10^{-3}$    | $7 \cdot 10^{-5}$               |
| 2.3         | $6.17 \cdot 10^{-3}$    | $6 \cdot 10^{-5}$               |
| 2.5         | $6.31 \cdot 10^{-3}$    | $5 \cdot 10^{-5}$               |
| 2.8         | $6.68 \cdot 10^{-3}$    | $5 \cdot 10^{-5}$               |
| 3.1         | $6.98 \cdot 10^{-3}$    | $5 \cdot 10^{-5}$               |
| 3.4         | $7.37 \cdot 10^{-3}$    | $4 \cdot 10^{-5}$               |
| 3.7         | $7.83 \cdot 10^{-3}$    | $4 \cdot 10^{-5}$               |
| 4.0         | $8.42 \cdot 10^{-3}$    | $4 \cdot 10^{-5}$               |
| 4.2         | $9.11 \cdot 10^{-3}$    | $5 \cdot 10^{-5}$               |
| 4.5         | $1.00 \cdot 10^{-2}$    | $5 \cdot 10^{-5}$               |
| 4.8         | $1.13 \cdot 10^{-2}$    | $5 \cdot 10^{-5}$               |
| 5.1         | $1.31 \cdot 10^{-2}$    | $6 \cdot 10^{-5}$               |
| 5.4         | $1.51 \cdot 10^{-2}$    | $6 \cdot 10^{-5}$               |
| 5.7         | $1.83 \cdot 10^{-2}$    | $6 \cdot 10^{-5}$               |
| 5.9         | $2.28 \cdot 10^{-2}$    | $8 \cdot 10^{-5}$               |
| 6.2         | $2.90 \cdot 10^{-2}$    | $1 \cdot 10^{-4}$               |
| 6.5         | $3.48 \cdot 10^{-2}$    | $1 \cdot 10^{-4}$               |
| 6.8         | $3.46 \cdot 10^{-2}$    | $1 \cdot 10^{-4}$               |
| 7.1         | $2.50 \cdot 10^{-2}$    | $7 \cdot 10^{-5}$               |
| 7.4         | $1.32 \cdot 10^{-2}$    | $4 \cdot 10^{-5}$               |
| 7.6         | $6.14 \cdot 10^{-3}$    | $2 \cdot 10^{-5}$               |
| 7.9         | $2.68 \cdot 10^{-3}$    | $8 \cdot 10^{-6}$               |
| 8.2         | $1.03 \cdot 10^{-3}$    | $3 \cdot 10^{-6}$               |
| 8.5         | $3.23 \cdot 10^{-4}$    | $1 \cdot 10^{-6}$               |
| 8.8         | $5.28 \cdot 10^{-5}$    | $2 \cdot 10^{-7}$               |
| 9.1         | $8.60 \cdot 10^{-6}$    | $5 \cdot 10^{-8}$               |
| 9.3         | $8.62 \cdot 10^{-5}$    | $3 \cdot 10^{-7}$               |
| 9.6         | $2.36 \cdot 10^{-4}$    | $6 \cdot 10^{-7}$               |
| 9.9         | $4.28 \cdot 10^{-4}$    | $9 \cdot 10^{-7}$               |
| 10.2        | $6.47 \cdot 10^{-4}$    | $2 \cdot 10^{-6}$               |
| 10.5        | $8.86 \cdot 10^{-4}$    | $2 \cdot 10^{-6}$               |

|      |                      |                   |
|------|----------------------|-------------------|
| 10.8 | $1.14 \cdot 10^{-3}$ | $2 \cdot 10^{-6}$ |
| 11.0 | $1.39 \cdot 10^{-3}$ | $3 \cdot 10^{-6}$ |
| 11.3 | $1.63 \cdot 10^{-3}$ | $3 \cdot 10^{-6}$ |
| 11.6 | $1.84 \cdot 10^{-3}$ | $4 \cdot 10^{-6}$ |
| 11.9 | $1.98 \cdot 10^{-3}$ | $4 \cdot 10^{-6}$ |
| 12.2 | $2.01 \cdot 10^{-3}$ | $4 \cdot 10^{-6}$ |
| 12.5 | $1.93 \cdot 10^{-3}$ | $4 \cdot 10^{-6}$ |
| 12.7 | $1.74 \cdot 10^{-3}$ | $4 \cdot 10^{-6}$ |
| 13.0 | $1.46 \cdot 10^{-3}$ | $3 \cdot 10^{-6}$ |
| 13.3 | $1.16 \cdot 10^{-3}$ | $2 \cdot 10^{-6}$ |
| 13.6 | $8.60 \cdot 10^{-4}$ | $2 \cdot 10^{-6}$ |
| 13.9 | $5.90 \cdot 10^{-4}$ | $2 \cdot 10^{-6}$ |
| 14.2 | $3.66 \cdot 10^{-4}$ | $1 \cdot 10^{-6}$ |
| 14.4 | $2.02 \cdot 10^{-4}$ | $6 \cdot 10^{-7}$ |
| 14.7 | $9.56 \cdot 10^{-5}$ | $3 \cdot 10^{-7}$ |
| 15.0 | $3.34 \cdot 10^{-5}$ | $2 \cdot 10^{-7}$ |
| 15.3 | $5.09 \cdot 10^{-6}$ | $4 \cdot 10^{-8}$ |
| 15.6 | $2.19 \cdot 10^{-6}$ | $2 \cdot 10^{-8}$ |
| 15.9 | $1.74 \cdot 10^{-5}$ | $1 \cdot 10^{-7}$ |
| 16.1 | $4.59 \cdot 10^{-5}$ | $2 \cdot 10^{-7}$ |
| 16.4 | $8.61 \cdot 10^{-5}$ | $5 \cdot 10^{-7}$ |
| 16.7 | $1.29 \cdot 10^{-4}$ | $9 \cdot 10^{-7}$ |
| 17.0 | $1.75 \cdot 10^{-4}$ | $1 \cdot 10^{-6}$ |
| 17.3 | $2.30 \cdot 10^{-4}$ | $2 \cdot 10^{-6}$ |
| 17.6 | $2.71 \cdot 10^{-4}$ | $2 \cdot 10^{-6}$ |

TABLE IV: Spectral density (i.e., the Fourier transform of the covariance  $\chi_V(r) = S_2(r) - \phi^2$ ) of MRJ hard-sphere packings. It is derived from the direct Fourier transformation of the periodic simulation box. The allowed values of the wave vector are binned w.r.t. their absolute value  $k$  and the resulting spectral densities are then averaged over 14 different packings. The third column displays the standard error of the mean.

| $k \cdot D$ | $\tilde{\chi}_V(k)/D^3$ | $\sigma[\tilde{\chi}_V(k)]/D^3$ |
|-------------|-------------------------|---------------------------------|
| 0.3         | $3.70 \cdot 10^{-4}$    | $1 \cdot 10^{-4}$               |
| 0.6         | $9.36 \cdot 10^{-4}$    | $9 \cdot 10^{-5}$               |
| 0.9         | $1.39 \cdot 10^{-3}$    | $2 \cdot 10^{-4}$               |
| 1.2         | $1.63 \cdot 10^{-3}$    | $2 \cdot 10^{-4}$               |
| 1.5         | $1.86 \cdot 10^{-3}$    | $1 \cdot 10^{-4}$               |
| 1.8         | $2.29 \cdot 10^{-3}$    | $1 \cdot 10^{-4}$               |
| 2.1         | $2.70 \cdot 10^{-3}$    | $2 \cdot 10^{-4}$               |
| 2.4         | $2.43 \cdot 10^{-3}$    | $2 \cdot 10^{-4}$               |
| 2.7         | $2.83 \cdot 10^{-3}$    | $1 \cdot 10^{-4}$               |
| 3.0         | $2.96 \cdot 10^{-3}$    | $2 \cdot 10^{-4}$               |
| 3.3         | $3.03 \cdot 10^{-3}$    | $2 \cdot 10^{-4}$               |
| 3.6         | $3.39 \cdot 10^{-3}$    | $9 \cdot 10^{-5}$               |
| 3.9         | $3.25 \cdot 10^{-3}$    | $8 \cdot 10^{-5}$               |
| 4.2         | $3.83 \cdot 10^{-3}$    | $1 \cdot 10^{-4}$               |
| 4.5         | $4.07 \cdot 10^{-3}$    | $7 \cdot 10^{-5}$               |
| 4.8         | $4.37 \cdot 10^{-3}$    | $9 \cdot 10^{-5}$               |

|      |                      |                   |
|------|----------------------|-------------------|
| 5.1  | $5.01 \cdot 10^{-3}$ | $1 \cdot 10^{-4}$ |
| 5.4  | $5.55 \cdot 10^{-3}$ | $2 \cdot 10^{-4}$ |
| 5.7  | $6.89 \cdot 10^{-3}$ | $2 \cdot 10^{-4}$ |
| 6.0  | $8.10 \cdot 10^{-3}$ | $2 \cdot 10^{-4}$ |
| 6.3  | $1.05 \cdot 10^{-2}$ | $2 \cdot 10^{-4}$ |
| 6.6  | $1.38 \cdot 10^{-2}$ | $4 \cdot 10^{-4}$ |
| 6.9  | $1.93 \cdot 10^{-2}$ | $5 \cdot 10^{-4}$ |
| 7.2  | $2.35 \cdot 10^{-2}$ | $7 \cdot 10^{-4}$ |
| 7.5  | $2.28 \cdot 10^{-2}$ | $4 \cdot 10^{-4}$ |
| 7.8  | $1.34 \cdot 10^{-2}$ | $4 \cdot 10^{-4}$ |
| 8.1  | $4.53 \cdot 10^{-3}$ | $1 \cdot 10^{-4}$ |
| 8.4  | $1.10 \cdot 10^{-3}$ | $4 \cdot 10^{-5}$ |
| 8.7  | $1.91 \cdot 10^{-4}$ | $7 \cdot 10^{-6}$ |
| 9.0  | $9.28 \cdot 10^{-6}$ | $5 \cdot 10^{-7}$ |
| 9.3  | $9.12 \cdot 10^{-5}$ | $4 \cdot 10^{-6}$ |
| 9.6  | $2.37 \cdot 10^{-4}$ | $6 \cdot 10^{-6}$ |
| 9.9  | $4.18 \cdot 10^{-4}$ | $7 \cdot 10^{-6}$ |
| 10.2 | $6.03 \cdot 10^{-4}$ | $1 \cdot 10^{-5}$ |
| 10.5 | $7.78 \cdot 10^{-4}$ | $2 \cdot 10^{-5}$ |
| 10.8 | $9.67 \cdot 10^{-4}$ | $2 \cdot 10^{-5}$ |
| 11.1 | $1.18 \cdot 10^{-3}$ | $2 \cdot 10^{-5}$ |
| 11.4 | $1.35 \cdot 10^{-3}$ | $2 \cdot 10^{-5}$ |
| 11.7 | $1.49 \cdot 10^{-3}$ | $2 \cdot 10^{-5}$ |
| 12.0 | $1.69 \cdot 10^{-3}$ | $3 \cdot 10^{-5}$ |
| 12.3 | $1.86 \cdot 10^{-3}$ | $2 \cdot 10^{-5}$ |
| 12.6 | $2.02 \cdot 10^{-3}$ | $2 \cdot 10^{-5}$ |
| 12.9 | $2.03 \cdot 10^{-3}$ | $2 \cdot 10^{-5}$ |
| 13.2 | $1.86 \cdot 10^{-3}$ | $2 \cdot 10^{-5}$ |
| 13.5 | $1.57 \cdot 10^{-3}$ | $1 \cdot 10^{-5}$ |
| 13.8 | $1.11 \cdot 10^{-3}$ | $1 \cdot 10^{-5}$ |
| 14.1 | $7.17 \cdot 10^{-4}$ | $6 \cdot 10^{-6}$ |
| 14.4 | $4.13 \cdot 10^{-4}$ | $3 \cdot 10^{-6}$ |
| 14.7 | $1.89 \cdot 10^{-4}$ | $3 \cdot 10^{-6}$ |
| 15.0 | $6.08 \cdot 10^{-5}$ | $1 \cdot 10^{-6}$ |
| 15.3 | $7.72 \cdot 10^{-6}$ | $2 \cdot 10^{-7}$ |
| 15.6 | $5.31 \cdot 10^{-6}$ | $2 \cdot 10^{-7}$ |
| 15.9 | $2.93 \cdot 10^{-5}$ | $5 \cdot 10^{-7}$ |
| 16.2 | $6.41 \cdot 10^{-5}$ | $7 \cdot 10^{-7}$ |
| 16.5 | $1.05 \cdot 10^{-4}$ | $9 \cdot 10^{-7}$ |
| 16.8 | $1.41 \cdot 10^{-4}$ | $1 \cdot 10^{-6}$ |
| 17.1 | $1.83 \cdot 10^{-4}$ | $2 \cdot 10^{-6}$ |
| 17.4 | $2.17 \cdot 10^{-4}$ | $2 \cdot 10^{-6}$ |
| 17.7 | $2.64 \cdot 10^{-4}$ | $3 \cdot 10^{-6}$ |
| 18.0 | $2.99 \cdot 10^{-4}$ | $5 \cdot 10^{-6}$ |
| 18.3 | $3.31 \cdot 10^{-4}$ | $4 \cdot 10^{-6}$ |
| 18.6 | $3.77 \cdot 10^{-4}$ | $4 \cdot 10^{-6}$ |
| 18.9 | $3.96 \cdot 10^{-4}$ | $5 \cdot 10^{-6}$ |
| 19.2 | $4.08 \cdot 10^{-4}$ | $8 \cdot 10^{-6}$ |
| 19.5 | $3.81 \cdot 10^{-4}$ | $6 \cdot 10^{-6}$ |
